# Supplementary material for: Extended Magnetic Exchange Interactions in the High-Temperature Ferromagnet MnBi
Source: arXiv:1603.02750 source file (2016-03-10)
Supplement: Supplementary file 1 [file MnBi_supplemental.pdf]

# Supplemental Information for Williams et al. *Extended Magnetic Exchange Interactions in the High-Temperature Ferromagnet MnBi*

## I. DATA FITTING PROCEDURE

The data was fit to a Heisenberg model given by:

$$H = J_n \sum_{<i,j>} \mathbf{S_i} \cdot \mathbf{S_j} \qquad (1)$$

where $J_n$ is the exchange interaction between the $n$-th nearest neighbors $S_i$ and $S_j$, taking the convention that positive values of $J_n$ denote antiferromagnetic exchange. In order to parametrize the data we needed to include nearest-neighbors out to $d$ = 7.5 Å, which requires exchange interactions up to $J_6$. Fits using fewer exchange constants did not reproduce the data, particularly along ($H$ 0 1) (shown in Fig. S1(d)) where the $6^{th}$ nearest neighbor term contributes an additional sinusoidal term.

Constant-$Q$ cuts were made through the data and the cuts were fit to a Gaussian to extract the peak energy for each cut. This array of 25 points were taken from the following directions: ($H$ 0 $\frac{1}{2}$), ($H$ 0 2), ($H$ 0 3), ($\frac{1}{2}$ 0 L), (1 0 L), and (2 0 L). The results of the fitting gave the values of the exchange constants listed in Table I of the Letter. The errors were calculated by the method described in[1]. Using these values, the data was simulated to produce plots of $S(Q,\omega)$ shown in Fig.S1, below.

No resolution corrections were included in the fits, but the plots below have been convoluted with a two-dimensional Gaussian function to approximate the energy- and $Q$-resolution of the instrument. The magnetic form factor is also included in these plots.

## II. FIRST PRINCIPLES CALCULATIONS

The principal question theory should answer regarding MnBi is the following: how is it possible that in a magnetic material containing Manganese - which usually prefers antiferromagnetic behavior - ferromagnetic behavior arises, and most crucially, *how does ferromagnetic behavior arise despite the nearest neighbor Mn-Mn coupling being antiferromagnetic*?

To understand the magnetic behavior of MnBi, we have performed first principles calculations of the effective Heisenberg exchange parameters $J_{ij}$. using the generalized gradient approximation (GGA)[2] in the planewave all-electron density functional theory code WIEN2K[3]. One recalls that in such a Heisenberg model, usually applicable to systems such as MnBi where the magnetic element carries a sizable local moment, the system energy can be taken (relative to a zero of energy) as

$$E = \sum_{<i,j>} J_{i,j} \mathbf{S_i} \cdot \mathbf{S_j} \qquad (2)$$

where the $< i, j >$ represent first, second, etc. nearest neighbors and it is presumed that a single $J_{i,j}$ is applicable to all atom neighbor pairs $< i, j >$ of equal separation. Here the **S** represent the Pauli spin-operators. Note that while in Eq. 1 the magnitude of the spin (i.e. $S(S+1)$) enters, in the following paragraphs we treat S(S+1) as unity; to extract actual $J_{i,j}$ values one should divide by 3.77*(3.77+1) $\sim$ 18 (since the calculated Mn spin moment is approximately 3.77 $\mu_B$.)

The results of the calculations are as follows. Firstly, in agreement with experiment, of all the configurations modeled the ferromagnetic case has the lowest energy. The simplest antiferromagnetic case, in which the Mn-Mn nearest neighbors along the c-axis are anti-aligned, lies some 135 meV ($\sim \Delta E$) per Mn higher, leading to a mean-field Curie point estimate $T_c = \Delta E/3 = 522K$, in reasonable agreement with the experimental value of 630 K. Also in agreement with experiment, the nearest-neighbor $J_1$= 4.22 meV, indicating a tendency towards *antiferromagnetic* alignment. The second nearest-neighbor (the in-plane nearest-neighbor), $J_2$ at 1.74 meV is also positive. However, $J_3$-$J_6$ are all negative, and in particular $J_3$ is -6.33 meV and $J_5$ is -8.33 meV. Given that these last two J's comprise 12 and 6 neighbor pairs, respectively, the combination of these exchange constants provides an energy incentive of over 100 meV per Mn for ferromagnetic alignment, which in the calculations is the "driving force" for ferromagnetism in MnBi. The NiAs hexagonal structure, with its large number of Mn-Mn distant neighbors and relatively small (2) number of nearest neighbors is clearly of great importance for the ferromagnetism.

---


1 P.R. Bevington and D.K. Robinson, *Data Reduction and Error Analysis for the Physical Sciences*. 3rd. Ed. (McGraw-Hill, New York, New York, USA, 2003).

2 J.P. Perdew, K. Burke, and M. Ernzerhof, Generalized gradient approximation made simple, Phys. Rev. Lett. **77** , 3865 (1996).

3 P. Blaha, K, Schwarz, G. Madsen, D, Kvasnicka and J. Luitz, WIEN2k, An Augmented Plane Wave + Local Orbitals Program for Calculating Crystal Properties (K. Schwarz, Tech. Univ. Wien, Austria, 2001).

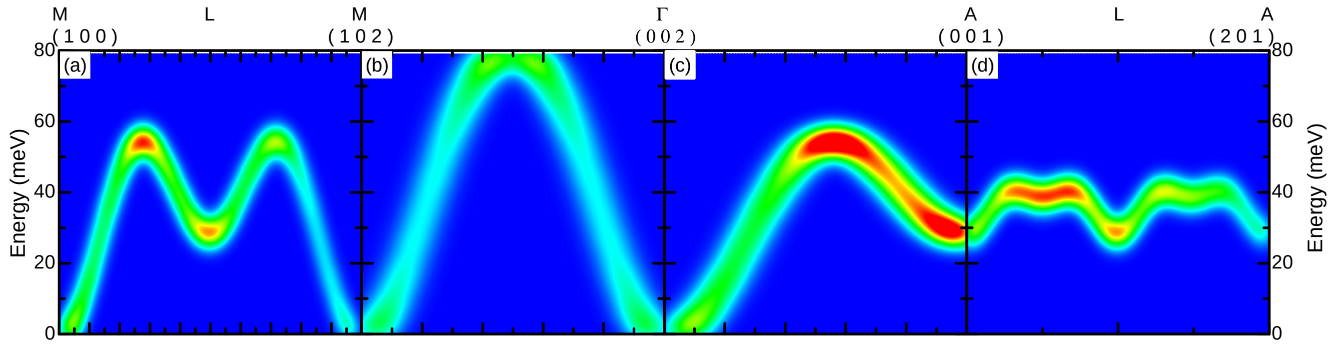


FIG. S1. (Color online) Simulations of the data based on the exchange constants found in the fitting procedure described above, shown along the same directions in reciprocal space as the data in Fig. 2(a) to (d) of the Letter. The instrumental resolution has been been included by convolving the fit with a two-dimensional Gaussian, and the magnetic form factor has also been applied.
